# Supplementary material for: Seeing Beyond 8bits: Subjective and Objective Quality Assessment of HDR-UGC Videos
Source: arXiv:2603.00938 source file (2026-03-01)
Supplement: Supplementary file 1 [file supp_appendix.tex]

%%%%%%%%%%%%%%%%%%%%%%%%%%%%%%%%%%%%%%%%%%%%%%%%%%%%%%%%%%%%%%%%%%%%%%%%%%%%%%%
% APPENDIX
%%%%%%%%%%%%%%%%%%%%%%%%%%%%%%%%%%%%%%%%%%%%%%%%%%%%%%%%%%%%%%%%%%%%%%%%%%%%%%%
\clearpage
\appendix
\onecolumn

\tableofcontents

\newpage

\section{Appendix}

This supplementary material expands on the technical, experimental, and ethical components of \textcolor{hdrblue}{\textbf{HDR-Q}} that could not be included in the main paper due to space constraints. It provides additional dataset details, methodological clarification, and extended empirical analysis to fully support the claims made in the primary manuscript.

% \begin{itemize}
%     \item \textbf{Related Work:} Extended discussion of HDR-VQA and MLLM-based perceptual quality literature.
%     \item \textbf{Dataset Details:} Comprehensive documentation of collection pipeline, AMT protocol, QC procedures, HDR verification, reliability analyses, and MOS behaviors.
%     \item \textbf{Dataset Analysis:} Content diversity, SI–TI characteristics, MOS distributions, bitrate–resolution trends, and demographic insights.
%     \item \textbf{Method Details:} Additional exposition of HAPO, reward design, two-stage RL training, and HDR-aware encoder formulation.
%     \item \textbf{Qualitative Examples:} Additional visualizations of reasoning output of our model. 
%     \item \textbf{Ethical Considerations:} Discussion of privacy, dataset usage constraints, bias, and responsible deployment.
% \end{itemize}

\section{Related Work}
\label{app:related_work}

\subsection{HDR-VQA: Datasets and Models}
Subjective video quality datasets such as CVD2014~\citep{CVD2014}, LIVE-VQA~\citep{LIVEVQA}, LIVE-VQC~\citep{LIVE-VQC}, LSVQ~\citep{LSVQ}, MDVQA~\citep{MDVQA}, and Maxwell~\citep{maxwell} have driven progress in SDR VQA by supporting the development of handcrafted models~\citep{NIQE,BRISQUE,V-BLINDS,TLVQM,VIIDEO,ChipQA} and deep learning architectures~\citep{VSFA,FASTVQA,FASTERVQA,CONTRIQUE,cover,Dover}. These datasets however operate entirely in SDR, with limited luminance ranges and no notion of PQ-transfer or wide color gamut content, making them insufficient for algorithms intended to handle HDR-specific perceptual phenomena. To address HDR scenarios, several early HDR VQA datasets were introduced~\citep{azimi2021pu21,pan2018hdr,baroncini2016verification,rerabek2015subjective,athar2019perceptual}. Many of these collections involve small content diversity, outdated HDR standards, or limited accessibility, which restricts their modern usability. LIVE-HDR~\citep{LIVE-HDR} provides a more contemporary benchmark with 310 annotated clips generated under controlled distortions. SFV+HDR~\citep{sfv+hdr} expands toward short-form user content with 2k clips, yet only 300 are annotated due to high labeling cost. The field therefore lacks sufficiently large, diverse HDR datasets capturing practical user-generated conditions, tone-mapping inconsistencies, sensor noise, or extreme dynamic-range variation. Parallel to dataset development, several HDR VQA algorithms have been proposed. Full-reference metrics such as HDR-VQM~\citep{HDR-VQM}, HDR-BVQM~\citep{HDR-BVQM}, and PU21~\citep{PU21} leverage perceptually uniform luminance transforms or brightness-adaptive operators. These methods however assume pristine references and are not suited to the unpredictable variability of UGC. Blind HDR models emerged more recently. HDR-ChipQA~\citep{HDR-ChipQA} extends ChipQA with nonlinear luminance modeling, while HIDRO-VQA~\citep{HIDRO-VQA} adapts CONTRIQUE~\citep{CONTRIQUE} through large-scale pretraining on unlabeled YouTube HDR videos. Although these approaches incorporate HDR-specific priors, they do not robustly handle HDR-UGC distortions such as clipped highlights, crushed shadows, quantization banding, or gamut shifts that dominate modern consumer-captured HDR. This motivates the construction of larger HDR-UGC datasets and more principled modeling frameworks capable of reasoning about HDR-specific perceptual cues.

\subsection{MLLM-Based Perceptual Quality Assessment}
Multimodal large language models have increasingly been applied to perceptual quality assessment. Q-Bench~\citep{qbench} established that general-purpose MLLMs remain far from human perception, with large inconsistencies in both ranking and scoring tasks. Instruction tuning approaches such as Q-Instruct~\citep{qinstruct} and Q-Bench’s instruction-aligned variants improved distortion awareness by coupling low-level quality cues with textual descriptions. DepictQA~\citep{depictqa} and DepictQA-Wild~\citep{depictqawild} moved toward more naturalistic distortion explanations by prompting models to produce descriptive rationales before scoring. Several studies have proposed more structured formulations. Compare2Score~\citep{compare2score} demonstrated that pairwise comparison signals are easier for MLLMs to model and can be meta-learned to form continuous scores. Reinforcement learning-to-rank was explored in VisualQuality-R1~\citep{visualquality}, which improved alignment with human preferences. Discrete quality level calibration methods such as Q-Align~\citep{qalign} improved robustness but sacrificed continuous regression fidelity. DeQA-Score~\citep{deqa} incorporated multi-dataset training with soft labels to better capture MOS distributions. Q-Insight~\citep{qinsight} used reinforcement learning to improve joint score prediction and degradation perception.

\noindent
Video-focused extensions include Q-Bench-Video~\citep{qbenchvideo}, which provided the first unified benchmark for evaluating MLLMs on spatiotemporal distortions, and MVQA-68K~\citep{mvqa}, which introduced large-scale multi-attribute labels and textual rationales for training video-aware reasoning models. These works collectively point toward the feasibility of MLLMs for perceptual quality assessment, yet they remain fundamentally SDR-based. None explicitly address HDR, which involves different perceptual sensitivities, tone-mapping behaviors, and signal statistics. Moreover, existing approaches often rely on supervised or instruction tuning, whereas reinforcement learning for perceptual tasks is still in early stages.

\noindent
Our work extends this direction by introducing an HDR-aware vision encoder and a reinforcement learning framework explicitly optimized for HDR grounding, filling the gap between HDR-specific perception research and modern multimodal reasoning frameworks.

\section{Dataset Details}
\label{app:dataset}

\begin{figure*}[t]
    \centering
    \includegraphics[width=0.98\linewidth]{figs/exampleframes.drawio.jpg}
    \caption{Overview of our video dataset illustrated through sampled frames.}
    \label{fig:frames}
\end{figure*}

\subsection{Data Collection Sources}
As mentioned in the main paper, source videos were collected from:
\begin{itemize}
\item \textbf{Crowdsourcing Campaign:} An open call was made for users to submit HDR videos captured on their personal devices (various recent models of iPhones, Samsung Galaxy, Google Pixel, etc.). Submissions required user consent for research use. This yielded diverse, authentic UGC footage.
\item \textbf{Vimeo:} Videos licensed under Creative Commons were identified using Vimeo's search filters for HDR content. Manual screening ensured the videos were genuinely UGC (or representative of high-quality UGC) rather than professional productions. Categories included travel vlogs, personal events, amateur sports recordings, nature footage, etc.
\end{itemize}

Some example frames from our HDR video dataset are shown in Figure~\ref{fig:frames}.

\subsection{Video Filtering and Processing}
\begin{itemize}
    \item \textbf{Initial Filtering:} Automated checks removed videos with non-HDR flags, incompatible codecs, very low resolutions, or durations outside a reasonable range (e.g., $<$ 4s or $>$ 60s). Duplicate detection was performed. Manual screening removed clearly PGC content, static videos, and content violating ethical guidelines (privacy, safety).
    \item \textbf{Trimming:} Videos were trimmed to a maximum of 10 seconds, typically selecting a segment with representative motion and content complexity.
    \item \textbf{Bitrate Ladder Transcoding:} Using FFmpeg, source videos (considered 'Reference' quality) were transcoded to various resolution/bitrate combinations as specified in Table~\ref{tab:bitrate_ladder}. Encoding used HEVC Main 10 profile, with PQ transfer function and Rec.2020 color primaries, matching typical HDR10 standards. Constant Quality Rate Factor (CRF)was used to target the specified bitrates.
\end{itemize}

\begin{table}[ht]
\caption{Bitrate ladder used for dataset creation, simulating real-world streaming conditions~\citep{youtube_bitrate,apple_hls}. }
\vskip -0.2in
\label{tab:bitrate_ladder}
\vskip 0.15in
\begin{center}
\begin{small}
\begin{sc}
\begin{tabular}{lc}
\toprule
Resolution & Bitrates (Mbps) \\
\midrule
360p & 0.2, 0.5 \\ % Example values
720p & 0.5, 1.0, 2.0 \\ % Example values
1080p & 1.0, 2.0, 3.0, 5.0 \\ % Example values
1080p (Source) & Reference \\
\bottomrule
\end{tabular}
\end{sc}
\end{small}
\end{center}
\vskip -0.1in
\end{table}

\subsection{Crowdsourced Subjective Study}
\label{sec:subjective}
We conducted a large-scale crowdsourced study on Amazon Mechanical Turk (AMT) to collect human quality judgments for HDR user-generated content (HDR-UGC), adapting best practices from prior work on crowdsourced video quality assessment~\citep{AMT1,AMT2,LSVQ,KVQ}. To address the unique challenges of remote HDR evaluation, we implemented strict device qualification (10bit HDR Display, HDR playback capable browser, stable internet, etc.), persistent HDR capability checks, multi-stage quality control, and robust score aggregation.

\begin{figure}[ht]
    \centering
    % Subfigure 1
    \includegraphics[width=0.98\linewidth]{figs/main.png}
    \caption{General instruction of this study on AMT}
    \label{fig:main}
\end{figure}

\begin{figure}[ht]
    \centering
    % Subfigure 1
    \includegraphics[width=0.98\linewidth]{figs/howto.png}
    \caption{Rating instructions on AMT.}
    \label{fig:howto}
\end{figure}

\begin{figure}[h!]
    \centering
    % Subfigure 1
    \includegraphics[width=0.95\linewidth]{figs/quiz.png}
    \caption{Quiz phase on AMT.}
    \label{fig:mturk-quiz}
\end{figure}

\begin{figure}[ht]
    \centering
    % Subfigure 1
    \includegraphics[width=0.98\linewidth]{figs/train-test-instuction.png}
    \caption{Train-test Instruction phase on AMT.}
    \label{fig:train}
\end{figure}

\begin{figure}[ht]
    \centering
    % Subfigure 1
    \includegraphics[width=0.98\linewidth]{figs/ethics.png}
    \caption{Ethics policy on AMT.}
    \label{fig:ethics}
\end{figure}

\subsection{Platform and Participants}
\textbf{Platform.} AMT was used as the crowdsourcing platform.\\
\textbf{Geography and compensation.} We primarily recruited workers from regions with higher HDR device penetration (e.g., North America and Europe). Compensation was set above typical local minimum wage for the estimated task duration.\\
\textbf{Eligibility and qualification.} Workers had to pass a multi-part qualification: (i) verification of HDR10-capable display, (ii) stable internet connection, (iii) English instruction comprehension, and (iv) a short training/quiz on the rating task (examples and multiple-choice questions), see Fig.~\ref{fig:mturk-quiz}. Only workers who passed all checks were admitted to the main study.

\subsection{Stimuli and HIT Design}
The main instructions of the study shown in Fig.~\ref{fig:main}. Each Human Intelligence Task (HIT) presented a batch of videos in a custom web interface capable of rendering HDR content leveraging browser support. Playback controls were limited to play/pause and replay; seeking was disabled to ensure that the entire clip was viewed prior to rating. Subjects used a likert-scale (0--100) to provide quality scores (rating instructions shown in Fig.~\ref{fig:howto}). 

\subsection{HDR Capability Verification}
Ensuring true HDR playback is critical for data validity. We implemented:
\begin{itemize}
    \item \textbf{Pre-screening:} Client-side scripts probed display and browser capabilities indicative of HDR10 playback (e.g., bit depth, EOTF/codec support, and resolution proxies).
    \item \textbf{Persistent checks:} The same probes were re-run periodically during the HIT (e.g., at section boundaries) to detect display or window changes mid-task.
\end{itemize}
Workers whose devices failed initial or persistent checks were disqualified; ratings collected during failed sessions were discarded.

\noindent
\textbf{Training phase.} Before the main test, subjects rated six HDR videos to familiarize themselves with the interface and the intended use of the likert-scale scale (Fig.~\ref{fig:train}). Feedback and brief reminders reinforced proper use of the range.

\noindent
\textbf{Testing phase.} Each participant then rated 94 videos. To monitor consistency and calibration, we embedded five golden-set videos (with MOS obtained from lab/pilot studies) and five repeat (duplicate) videos within the test set. Across the full dataset, each video received on average $\sim$35 ratings.

\subsection{Quality Control (QC)}
We combined a priori design constraints with a posteriori checks:
\begin{itemize}
    \item \textbf{Golden-set agreement:} Ratings deviating by more than two standard deviations from pilot MOS were flagged.
    \item \textbf{Repeat consistency:} For duplicated videos, absolute differences $>$ 20 points indicated inconsistency.
    \item \textbf{Timing anomalies:} Exceptionally fast or slow completion times (relative to clip length and page dwell) were flagged.
    \item \textbf{Playback integrity:} We monitored download stalls, abnormal replay patterns, and other playback issues. Progress checkpoints at $\sim$25\%, 50\%, and 75\% of the HIT facilitated mid-task intervention.
\end{itemize}

\noindent
\textbf{Rejection policy.} Participants exhibiting multiple QC failures (e.g., repeated golden-set deviations, excessive duplicate inconsistencies, or $>$50\% problematic playbacks) were disqualified and their ratings removed. Device-incompatible or non-HDR sessions were also rejected.

\subsection{Ethics and Privacy}
All workers provided informed consent within the AMT interface shown in Fig.~\ref{fig:ethics}. No personally identifiable information was stored beyond the minimum necessary for task operation and payment; HDR capability logs were retained only as anonymous technical flags for QC. The study design adhered to crowdsourcing ethics.% commonly adopted in prior VQA datasets.

\subsection{Reliability Analysis}
We assessed internal consistency and subject reliability using:
\begin{itemize}
    \item \textbf{Intra-subject repeatability:} We calculated the correlation between each subject's ratings on duplicate pairs and absolute repeat error. 
    \item \textbf{Inter-subject Correlation:} We randomly Split all MOS ratings into two independent groups and computed the Spearman Rank Correlation Coefficient (SRCC) and Pearson Linear Correlation Coefficient (PLCC) between them. The study achieved a median SRCC of 0.90 and a median PLCC of 0.92, shown in Fig.~\ref{fig:inter-sub}
\end{itemize}

\subsection{Summary of Scale and Outcomes}
In total, we processed $\sim$44K encoded sequences, each receiving on average $\sim$35 crowd ratings. After BT.500-style screening and SUREAL aggregation, we obtained robust MOS for HDR videos with associated confidence intervals. This constitutes, to our knowledge, the first crowdsourced large-scale HDR-UGC subjective study, designed to capture real-world device diversity while ensuring statistical reliability.

\begin{figure}[htbp]
    \centering
    \begin{subfigure}[b]{0.32\linewidth}
        \centering
        \includegraphics[width=0.8\linewidth]{figs/si-ti.png}
        \caption{SI vs. TI.}
        \label{fig:siti}
    \end{subfigure}
    \begin{subfigure}[b]{0.32\linewidth}
        \centering
        \includegraphics[width=0.8\linewidth]{figs/si-mos.png}
        \caption{MOS vs. SI.}
        \label{fig:mos-si}
    \end{subfigure}
    \begin{subfigure}[b]{0.32\linewidth}
        \centering
        \includegraphics[width=0.8\linewidth]{figs/ti-mos.png}
        \caption{MOS vs. TI.}
    \label{fig:mos-ti}
    \end{subfigure}
    \caption{(a) Spatial-Temporal Complexity, (b) MOS vs. Spatial Information (SI), and (c) MOS vs. Temporal Information (TI).}
    \label{fig:siti-figs}
\end{figure}

\section{Dataset Analysis}
\subsection{Content Analysis}
\textbf{SI-TI}: 
To better characterize the diversity of content complexity, Fig.~\ref{fig:siti-figs} provides an analysis of spatial-temporal complexity along with spatial information (SI) and temporal information (TI) in the dataset. The scatter plots in Fig.~\ref{fig:siti-figs} (a)–(c) highlight the variation in SI and TI values, revealing a broad range of texture and motion complexity. Higher SI values are associated with scenes containing rich textures and sharp edges, whereas higher TI values reflect sequences with fast motion or dynamic activity. The dataset encompasses both highly detailed static scenes and rapidly changing dynamic content, making it well-suited for assessing compression performance and HDR characteristics under diverse motion conditions.

\begin{figure}[htb]
    \centering
    % Subfigure 1
    \includegraphics[width=0.5\linewidth]{figs/inter-sub.png}
    \caption{Inter-subject correlation.}
    \label{fig:inter-sub}
\end{figure}

\subsection{MOS Analysis}
\textbf{MOS Distribution:}
Fig.~\ref{fig:mos} presents the distribution and CDF of mean scores across all videos. Fig.~\ref{fig:mos-dis-subfig1} shows the MOS distributions across video orientations, where landscape videos achieve higher scores on average than portrait videos.Fig.~\ref{fig:mos-dis-subfig2} illustrates the score distributions for Vimeo and Crowd. The orange histogram and curve represent Vimeo, while the purple histogram and curve represent Crowd, with probability density estimates shown as smooth lines.

\begin{figure}[htbp]
    \centering
    \begin{subfigure}[b]{0.45\linewidth}
        \centering
        \includegraphics[width=0.9\linewidth]{figs/mos.jpg}
        \caption{\centering MOS distribution.}
        \label{fig:mos-dis-sub1}
    \end{subfigure}
    \begin{subfigure}[b]{0.45\linewidth}
        \includegraphics[width=\linewidth]{figs/cdf.png}
        \caption{MOS CDF distribution.}
    \label{fig:mos-dis-sub2}
    \end{subfigure}
    \caption{(a) MOS distribution of all videos in UGC-HDR-44K. (b) MOS distributions of Vimeo and Crowd videos in UGC-HDR-44K.}
    \label{fig:mos}
\end{figure}

\begin{figure*}[htbp]
    \centering
    \begin{subfigure}[b]{0.45\textwidth}
        \centering
        \includegraphics[width=1\textwidth]{figs/landscape-portrait.jpg}
        \caption{\centering MOS Distribution for Portrait and Landscape.}
        \label{fig:mos-dis-subfig1}
    \end{subfigure}
    \begin{subfigure}[b]{0.45\textwidth}
        \includegraphics[width=1\textwidth]{figs/mos-dist.jpg}
        \caption{\centering MOS Distribution for Vimeo and Crowd.}
    \label{fig:mos-dis-subfig2}
    \end{subfigure}
    \caption{(a) MOS distribution of all videos in \textit{UGC-HDR-44K}. (b) MOS distributions of Vimeo and Crowd videos in \textit{UGC-HDR-44K}.}
    \label{fig:mos_distribution}
\end{figure*}

\noindent
\textbf{MOS vs. Bitrate ladders:}
Fig.~\ref{fig:mos-bitrateladder} presents the relationship between MOS and encoding parameters, namely bitrate and resolution, for both landscape and portrait videos. As shown in Fig.~\ref{fig:mos-bitrate} MOS consistently increases with higher bitrates, though the improvement plateaus at higher levels, with reference videos achieving the best quality. Similarly, Fig.~\ref{fig:mos-reso} demonstrates that higher resolutions lead to higher MOS, with 1080p and reference videos rated the highest. Across both analyses, landscape videos generally obtain slightly higher MOS than portrait videos, particularly at lower bitrates and resolutions. 

\begin{figure*}[htbp]
    \centering
    \begin{subfigure}[b]{0.45\linewidth}
        \centering
        \includegraphics[width=1\linewidth]{figs/mos_vs_bitrate.png}
        \caption{MOS vs. Bitrate.}
        \label{fig:mos-bitrate}
    \end{subfigure}
    \begin{subfigure}[b]{0.45\linewidth}
        \includegraphics[width=1\linewidth]{figs/mos_vs_resolution.png}
        \caption{MOS vs. Resolution.}
    \label{fig:mos-reso}
    \end{subfigure}
    \caption{(a) The MOS variations across bitrate. (2) The MOS variations across resolution.}
    \label{fig:mos-bitrateladder}
\end{figure*}

\begin{table}[t]
\centering
\setlength{\tabcolsep}{8pt}

\rowcolors{2}{panelbg}{white}
\begin{tabular}{>{\raggedright\arraybackslash}p{0.22\linewidth} >{\raggedright\arraybackslash}p{0.71\linewidth}}
\rowcolor{slate}\multicolumn{2}{l}{\bfseries\color{white} HDR UGC VQA: System Prompt Layout}\\

\rowcolor{hdrblue!12}\textbf{\color{slate} Role} &
\textbf{Expert in HDR video quality assessment, HDR perceptual evaluation. Evaluates full-video quality holistically.}\\

\rowcolor{sky!12}\textbf{\color{slate} Inputs} &
\texttt{[Video Frame]}, \texttt{[User Query / Context]}.\\

\rowcolor{amber!18}\textbf{\color{slate} Constraints} &
MOS must be a single integer (0–100).\\

\rowcolor{violet!12}\textbf{\color{slate} Output Tags} &
\texttt{<think>} Continuous reasoning \texttt{</think>}
then 
\texttt{<answer>mos</answer>}.\\

\end{tabular}
\caption{\textbf{Prompt Structure} for HDR UGC VQA under the updated system prompt.}
\label{tab:hdr_prompt_card}
\end{table}

\subsection{Dataset Limitations}
Limited motion features and distortion: we observed that collected HDR videos didn't have extereme motions in them as observed manually and confirmed from fig.~\ref{fig:siti-figs}.

\section{Method Details}
\label{app:method}
\subsection{HDR-Aware Policy Optimization (HAPO)}
\label{sec:hapo}
While GRPO~\citep{grpo} has proven effective for text-only reasoning tasks~\citep{yu2025dapo}, it offers no guarantee that the policy leverages perception cues effectively~\citep{papo}, rather than shortcutting through generic textual signals. This makes our task even more challenging which require us to capture HDR cues from input signals. To address this gap, we propose HDR-Aware Policy Optimization (HAPO), a reinforcement learning framework that explicitly enforces HDR grounding, stabilizes entropy, and improves credit assignment for reasoning-heavy HDR-UGC VQA.

\paragraph{HDR–SDR Contrastive KL.}
A key challenge in multimodal RL is modality neglect~\citep{modalityneglect}, where the model ignores modality-specific features if they are not explicitly rewarded~\citep{rafailov2023direct,modalityneglect}. In HDR-UGC VQA, this manifests as policies producing valid scores and rationales without exploiting HDR cues. Let $\pi_\theta^{\mathrm{HDR}}(\cdot)=\pi_\theta(\cdot\,|\,\text{text},v, v^{SDR})$ denote the policy conditioned on HDR, SDR, and text,$\pi_\theta^{\mathrm{SDR}}(\cdot)=\pi_\theta(\cdot\,|\,\text{text},v^{\mathrm{SDR}})$, the policy deprived of HDR video. In case of $\pi_\theta^{\mathrm{SDR}}$, we only give SDR video and text as input, and mask the HDR visual tokens in language decoder input space. Define:

\begin{equation}
\begin{aligned}
D_{\mathrm{KL}}\!\big(\pi_\theta^{\mathrm{HDR}} \,\|\, \pi_\theta^{\mathrm{SDR}}\big)
=
\mathbb{E}_{\{o_i\}\sim \pi_{\theta_{\mathrm{old}}}(\cdot|\text{text},v,v^{\mathrm{SDR}})}
\Bigg[
\frac{1}{K}\sum_{i=1}^{K} \frac{1}{|o_i|}
\sum_{t=1}^{|o_i|}
\left(
\frac{\pi_\theta^{\mathrm{HDR}}(o_{i,t})}{\pi_\theta^{\mathrm{SDR}}(o_{i,t})}
- \log\frac{\pi_\theta^{\mathrm{HDR}}(o_{i,t})}{\pi_\theta^{\mathrm{SDR}}(o_{i,t})}
- 1
\right)
\Bigg].
\label{eq:klhdr}
\end{aligned}
\end{equation}

\noindent
Maximizing $\mathcal{K}_{\mathrm{HDR}}$ ensures that removing HDR tokens significantly perturbs the decoding distribution, thereby incentivizing the model to exploit HDR-specific information rather than collapsing into SDR-only reasoning.

\subsection{Rewards}
\textbf{Format Reward ($R_{\mathrm{fmt}}$).} This reward encourages the model to generate reasoning outputs structured with the designated special token, i.e. using \texttt{<think>}..Reasoning..\texttt{</think>} and \texttt{<answer>}..Final Answer..\texttt{</answer>} tags, and it should be correctly follow a JSON format. 
\begin{equation}
R_{\mathrm{fmt}}=
\begin{cases}
1, & \text{if \textsc{Answer} adheres to the required format},\\[2pt]
0, & \text{otherwise.}
\end{cases}
\end{equation}
This prevents degenerate completions and guarantees that the policy remains aligned to the expected response template.

\noindent
\textbf{Score Reward ($R_{\mathrm{sc}}$).} Majority of existing reward formulations for image and video quality assessment use binary rewards~\citep{visualquality,qinsight}, assigning the same credit to all predictions within a threshold, ignoring their relative proximity to the ground truth. While some other uses linear L1-based rewards~\citep{deqa}, which improve upon binary reward but treat large and small errors with equal slope, offering little guidance once the model predictions are already close to accurate. All these methods provide only weak or coarse training signals, which leads to diminishing learning signals precisely in the regime where fine-grained calibration is most critical. Given perceptual quality assessment is inherently a regression problem, a more fitting reward would be that adjusts weight based on closeness to ground truth. Inspired from this, We introduce a gaussian weighted regression reward. The reward grows sharply as predictions approach the ground-truth MOS and gradually saturates near it, providing high-resolution feedback in the fine-grained regime while avoiding sensitivity to distant outliers. Formally, for predicted score $\hat{s}_i$ and ground truth $s_{\!*}$:
\begin{equation}
R_{\mathrm{sc}}(\hat{s}_i, s_{\!*})=\alpha \cdot \exp\!\left(-\frac{(\hat{s}_i-s_{\!*})^2}{2\sigma^2}\right),
\end{equation}
where $\sigma$ controls the tolerance to deviations and $\alpha \in (0,1]$ scales the overall magnitude. This formulation naturally emphasizes precision close to the target while still allowing coarse signals for distant errors, leading to more accurate and stable MOS predictions.

\noindent
\textbf{Self-Reward ($R_{\mathrm{self}}$).} Exploits within-group consensus. Given a group $\{o_i\}_{i=1}^K$, the majority answer $o^{\star}_{\mathrm{maj}}$ is identified:
\begin{equation}
o^{\star}_{\mathrm{maj}}=\arg\max_{o\in\{o_1,\ldots,o_K\}}\sum_{i=1}^K \mathbb{I}[o_i=o],
\end{equation}
and each response is rewarded as
\begin{equation}
R_{\mathrm{self}}(o_i)=\mathbb{I}[o_i=o^{\star}_{\mathrm{maj}}].
\end{equation}
This stabilizes learning when external verifiers are noisy and prevents vanishing-advantage issues. Finally, each completion $o_i=\langle \hat r,\hat s\rangle$ receives a total reward:
\begin{equation}
\mathcal{R}_i=w_{\mathrm{fmt}}R_{\mathrm{fmt}}
+w_{\mathrm{sc}}R_{\mathrm{sc}}
+w_{\mathrm{self}}R_{\mathrm{self}},
\end{equation}

\noindent
Together, these rewards jointly enforce structural validity, fine-grained MOS accuracy, HDR-aware attribute calibration, interpretable reasoning, and stable consensus-driven optimization.

\begin{figure*}[t]
    \centering
    \includegraphics[width=0.9\linewidth]{figs/appen-example.drawio.jpg}
    \caption{Visual Reasoning Sample.}
    \label{fig:example-reasone}
\end{figure*}

\subsection{Two-Stage Training Pipeline}
\label{sec:prelim:stages}
Our training follows a two-stage RL-based paradigm~\citep{qoq-med,sft-rl}, both optimized with the same objective but serving distinct purposes.

\noindent
\textbf{Stage~1: Modality Alignment.} Since HDR tokens and their projection layer are initialized from scratch, we first align the HDR-aware vision encoder, projection module, and the LLM decoder. Instead of conventional supervised fine-tuning (SFT), we employ the same HAPO-based training used in Stage~2. This ensures that from the outset the policy learns to integrate HDR tokens into the language input space while producing structured reasoning outputs. Such modality alignment stages are common in multimodal RL~\citep{yu2025dapo, papo}, where early grounding improves subsequent optimization.

\noindent
\textbf{Stage~2: Full RFT.} After alignment, we continue training on the full HDR-UGC corpus using the complete HAPO objective. This balances training across samples of varying distortion severity, improving MOS prediction, and HDR-aware reasoning quality. Unlike the conventional SFT followed by RL pipeline~\citep{sft-rl, rafailov2023direct}, both our stages use RL training, guaranteeing HDR grounding throughout.

\noindent
\textcolor{hdrblue}{\textbf{HDR-Q}} provides a unified framework for HDR-UGC quality assessment. First, the HDR-aware vision encoder produces tokens that are sensitive to extreme contrast, peak highlights, near-black detail, and wide color gamut properties unique to HDR content. Second, maximizing the HDR–SDR contrastive KL divergence forces the language decoding distribution to shift when HDR cues are removed, thereby increasing the conditional mutual information between outputs and HDR inputs. Third, policy entropy regularization suppresses trivial entropy inflation and stabilizes optimization. Fourth, high-entropy weighting (HEW) allocates stronger learning signals to explorative tokens, which are most critical for accurate artifact identification and quality calibration, addressing the credit assignment problem in reasoning. Finally, self-rewarding consolidates group consensus, reinforcing consistent rationales and calibrated MOS predictions across sampled responses, leading to stable and interpretable HDR-aware quality assessment.

\subsection{Ethical Considerations}
\label{app:ethics}
\begin{itemize}
    \item \textbf{Dataset Collection:} Videos collected through crowdsourcing involved explicit user consent for research purposes. Videos sourced from Vimeo were filtered for appropriate Creative Commons licenses. Efforts were made to filter personally identifiable information, though UGC content inherently carries privacy risks. The dataset will be released under a license restricting non-research use.
    \item \textbf{Subjective Study:} Participants were informed about the study's purpose and duration. Compensation was designed to be fair, exceeding typical platform rates. Data collected was anonymized. The study protocol was reviewed for ethical considerations regarding participant effort and potential exposure to diverse, unmoderated UGC.
    \item \textbf{Model Bias:} The dataset, despite efforts for diversity, may reflect biases present in the source platforms or participant demographics. The trained MLLM may inherit or amplify these biases. Potential biases related to perceived demographics, content types, or specific artifacts should be acknowledged.
    \item \textbf{Potential Misuse:} VQA models could potentially be used for unintended purposes, such as automated censorship or unfair content moderation. The focus of this work is perceptual quality assessment for improving user experience and system optimization.
\end{itemize}
